# Supplementary material for: Simulation of crack propagation through voxel-based, heterogeneous structures based on eigenerosion and finite cells
Source: arXiv:2202.10922 source file (2022-02-22)
Supplement: Supplementary file 1 [file sec_appendix.tex]

\section{This is a first Appendix \label{app:A}} 

This is the text of the first appendix. 

\section{This is the second Appendix}

This is the second appendix, the first one is given in Appendix~\ref{app:A}.
